# Supplementary material for: SENS: Semantic Synthetic Benchmarking Model for integrated supply chain simulation and analysis
Source: arXiv:2205.06484 source file (2022-05-13)
Supplement: Supplementary file 1 [file DemandFulfillment.tex]

\chapter{Demand Fulfillment  Queries}\label{demandfulffimentqueries}
\begin{lstlisting}[caption= Get Orders to Fulfill with OEM delivery time LT(O) ,label=alg_orders]
SELECT * WHERE {?ordr :hasDeliveryTime ?time. ?ordr :hasQuantity ?q. ?ordr :hasProduct ?p. ?cus :makes ?ordr. ?cus:hasPriority?prio.FILTER (?time-LT(O)=t)} ORDER BY DESC ?prio
\end{lstlisting}
\begin{lstlisting} [caption= Get OEM Inventory for Product P at time t,label=getinventory]
SELECT * WHERE { ?node a :OEM. ?node :hasInventory ?inv. ?inv :hasProduct :P. ?inv :hasTimeStamp "t". ?inv :hasQuantity ?q.}\end{lstlisting}

\begin{lstlisting} [caption= Generate Supply Plan for Order O for Product P at time t,label=generateplan]
INSERT { <<?SP :needsNode ?node>> :getsProduct :P <<?SP :neesNode ?node>> :hasTimeStamp :t
<<?SP :neesNode ?node>> :hasQuantity :q <<?SP :neesNode ?node>> :hasUnitPrice :price}
WHERE {:O :hasSupplyPlan ?SP. }
\end{lstlisting}

\begin{lstlisting} [caption= Get all Components for Product P,label=getcomponents ]
SELECT * WHERE { << :P :needsComponent ?comp >> :hasComponentQuantity ?quant.}
\end{lstlisting}

\begin{lstlisting} [caption= Get Supplier Capacity for Product P at time t,label=getsupplier, ]
SELECT * WHERE {?s :hasOEM :OEM1. ?s :hasCapacity ?cap. ?cap :hasProduct ?p. 
?cap :hasQuantity ?q. ?cap :hasTimeStamp ?ct. ?s :hasSaturation ?sat. ?s :hasLeadTime ?lt.
FILTER  (?sat>= ?q +  tofullfil) &&  (t - ?lt= ?ct).}
\end{lstlisting}

\raggedbottom
