# Supplementary material for: SENS: Semantic Synthetic Benchmarking Model for integrated supply chain simulation and analysis
Source: arXiv:2205.06484 source file (2022-05-13)
Supplement: Supplementary file 2 [file Evaluation_Appendix.tex]

\chapter{Evaluation Queries} \label{kpi}

\begin{table}[H]
\scriptsize
  \begin{tabular}{|p{.02\textwidth}|p{.51\textwidth}|p{.40\textwidth}|}

  % {@{}|l|c|c|@{}}
    \hline
    \bigstrut[t]      & SPARQL Query  & Result Sample  \\
    \hline
    \bigstrut[t] 
  \textit{Q1} & SELECT  \text{*} 
WHERE  \{   ?customer :makes ?order.\} & Node1.4 makes OrderJZHu5   
  \\\cline{1-3}

\textit{Q2} & SELECT  \text{*} 
WHERE \{  ?c a :Customer.  ?c2 a :Customer.  
?c ?x ?c2. \} & Node1.2 hasDwnStremNode Node2.3 
 \\\cline{1-3}

\textit{Q3} & SELECT \text{*} WHERE \{ 
<<:Product :needsProduct ?p>> :needsQuantity \} & <<ProductA needsProduct Product1>> needsQuantity 1 
\\\cline{1-3}

\textit{Q4}& SELECT \text{*} WHERE\{  :Node3.2 :hasProcess ?process. \}& :Node3.2 :hasProcess :PrcsA.
:PrcsA rdf:type :Make
\\\cline{1-3}

\textit{Q5} & SELECT   \text{*}  WHERE \{ 
:Node3.2 :hasSCORKPI ?kpi.\} & Responsiveness: 24 , Reliability: 85, Agility: 22 
\\\cline{1-3}

\textit{Q6}& SELECT \text{*} WHERE{ 
?node ?a :Node.}& Node1.1 :hasDownStreamNode 
Node1.2  
\\\cline{1-3}

%\textit{Q7}& Eliminated for conciseness  & Eliminated for conciseness 
%\\\cline{1-3}
%\textit{Q12}& Eliminated for conciseness  & Eliminated for conciseness 
%\\\cline{1-3}

   \end{tabular}
  \caption{SENS-SC Evaluation Queries and Corresponding Result Sample.}
  \label{evaluationqueries}
\end{table}

\raggedbottom
